# Supplementary material for: EntailE: Introducing Textual Entailment in Commonsense Knowledge Graph Completion
Source: arXiv:2402.09666 source file (2024-02-15)
Supplement: Supplementary file 1 [file 7-appendix.tex]

\section{Distribution and Ablation Study on ATOMIC}
\begin{figure}[t]
\centering
\includegraphics[scale=0.55,trim={0cm 0cm 0cm 1cm}]{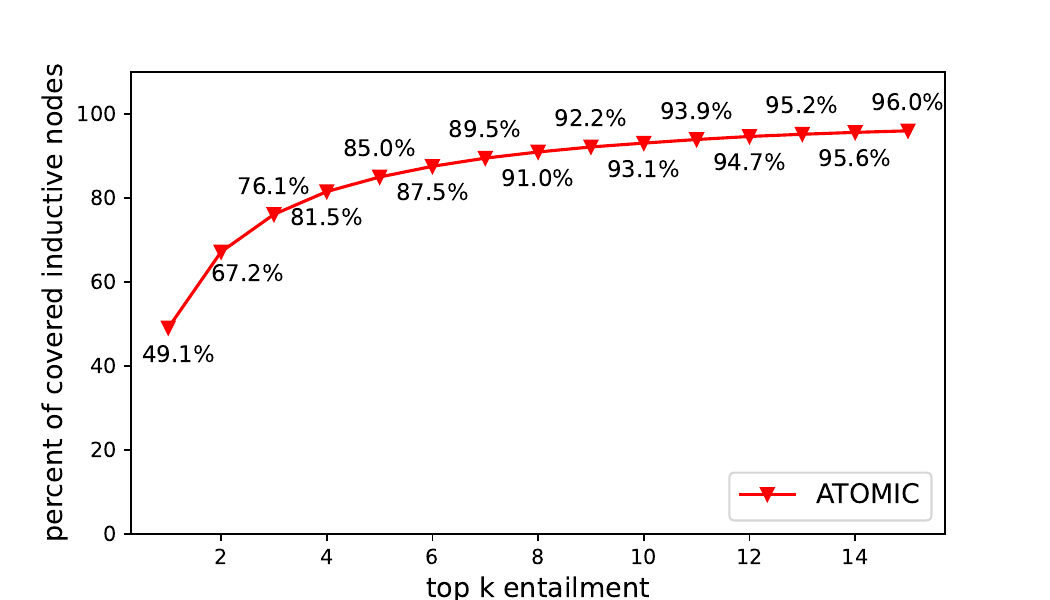}
\caption{Percentage of inductive ATOMIC nodes in the valid split covered by the entailment nodes of training split in ATOMIC. $k$ is the number of entailment nodes for each node in the training split.}
\vskip-0.5em
\label{append:1}
\end{figure}

\begin{table}[]
    \centering
    
    \caption{Ablation study of $\gamma_1$ on ATOMIC with EntailE. $k_1$=5, $\gamma_2=0.0$.}
    \label{append:2}
    \begin{tabular}{l|cccc}
    \toprule
    $\gamma_1$ & MRR & Hits@1 & Hits@3 & Hits@10 \\
    \midrule
    w/o entail & 13.74 & 10.80 & 14.42 & 19.48 \\
    \midrule
    %0.3 &  \\
    0.5 & \textbf{14.78} & \textbf{11.60} & \textbf{15.47} & \textbf{20.66}  \\
    1.0 & 14.06 & 10.97 & 14.61 & 19.89  \\
    \bottomrule
    \end{tabular}
    \vskip-1.5em
\end{table}

\begin{table}[]
    \centering
    
    \caption{Ablation study of $k_1$ on ATOMIC with EntailE. $\gamma_1=0.5, \gamma_2=0.0$.}
    \label{append:3}
    \begin{tabular}{l|cccc}
    \toprule
    $k$ & MRR & Hits@1 & Hits@3 & Hits@10 \\
    \midrule
    w/o entail & 13.74 & 10.80 & 14.42 & 19.48 \\
    \midrule
    %1 &  &  &  &  \\
    5 & \textbf{14.78} & \textbf{11.60} & \textbf{15.47} & \textbf{20.66}  \\
    %7 & \\
    10 & 14.14 & 10.98 & 14.90 & 20.06 \\
    \bottomrule
    \end{tabular}
    \vskip-1.5em
\end{table}

\subsection{Distribution of ATOMIC}
\label{appendixb}
The distribution of inductive nodes in valid split covered by training top $k$ entailed nodes is presented in Figure \ref{append:1}. It shows a similar trend with CN-82K. About 49\% Top-1 entailed nodes are included in the training nodes. With $k=10$, the coverage reaches up to 96\%, meaning almost all isolated node embeddings are updated. 

\subsection{$\gamma_1$ for ATOMIC}
The ablation study of $\gamma_1$ on ATOMIC is shown in Table \ref{append:2}.

\subsection{$k_1$ for ATOMIC}
The ablation study of $k_1$ on ATOMIC is shown in Table \ref{append:3}.
